# Supplementary material for: First-order tree-to-tree functions
Source: arXiv:2002.09307 source file (2023-01-30)
Supplement: Supplementary file 1 [file appendix-easy-combinators.tex]

\section{The easy combinators}

\subsection{Coproduct}
For each  ranked sets $\ranked{\Sigma_1}$, $\ranked{\Sigma_2}$  and $i \in \set{1,2}$, the $i$-th coprojection is defined by  
       \begin{align*}
           \ranked{\iota_i : \Sigma_i \to \Sigma_1 + \Sigma_2} \qquad   a \mapsto  (i,a)
       \end{align*}
       are defined by $\ranked{\iota_i}(a)= (i,a)$. Two arity preserving functions $\set{\ranked{f_i : \Sigma_i \to \Gamma}}_{i \in \set{1,2}}$ can be combined into a single function 
       \begin{align*}
           \ranked{\caseterm{f_1}{f_2} : (\Sigma_1 + \Sigma_2) \to \Gamma} \qquad (i,a) \mapsto \ranked{f_i}(a).
       \end{align*}

\subsection{Cartesian product}
For   ranked sets $\ranked{\Sigma_1}$, $\ranked{\Sigma_2}$ and $i \in \set{1,2}$, the $i$-th projection is defined by 
       \begin{align*}
           \ranked{\pi_i : \Sigma_1 \times \Sigma_2  \to \Sigma_i} \qquad (a_1,a_2) \mapsto a_i.
       \end{align*}
 Functions $\set{\ranked{f_i : \Sigma \to \Gamma_i}}_{i \in \set{1,2}}$ can be paired: 
       \begin{align*}
           \ranked{\pairfun{f_1}{f_2} : \Sigma \to  \Gamma_1 \times \Gamma_2} \qquad a \mapsto (\ranked{f_1}(a_1),\ranked{f_2}(a_2))
       \end{align*}
 Cartesian  product distributes across coproduct:
       \begin{align*}
           \ranked{\distrcart : (\Sigma_1 + \Sigma_2)\times \Gamma \to (\Sigma_1 \times \Gamma) + (\Sigma_2 \times \Gamma)}.
       \end{align*}
  
\subsection{Tensor product}

\datatypefigure
{
If $\ranked{\Sigma_1}$ and $\ranked{\Sigma_2}$ are ranked sets, then  their \emph{tensor product}
\begin{align*}
    \ranked{\Sigma_1 \product \Sigma_2}
\end{align*}
is also a ranked set. An $n$-ary element of the tensor product is a pair $\tensorpair {a_1,a_2}$ such that $a_i \in \ranked{\Sigma_i}$ and 
\begin{align*}
    n = \arity{a_1} + \arity{a_2}.
\end{align*}
We use angled brackets to distinguish tensor pairs $\tensorpair{a_1,a_2}$ from Cartesian pairs $(a_1,a_2)$. 
}
{
       \item Functions $\set{\ranked{f_i : \Sigma_i \to \Gamma_i}}_{i \in \set{1,2}}$ can tensored: 
       \begin{align*}
           \ranked{\tensorfun{f_1}{f_2} : \Sigma_1 \product \Sigma_2 \to  \Gamma_1 \product \Gamma_2}
       \end{align*}
       \item Tensor  product distributes across coproduct:
       \begin{align*}
           \ranked{\distrtensor : (\Sigma_1 + \Sigma_2)\product \Gamma \to (\Sigma_1 \product \Gamma) + (\Sigma_2 \product \Gamma)}.
       \end{align*} 
}
