# Supplementary material for: First-order tree-to-tree functions
Source: arXiv:2002.09307 source file (2023-01-30)
Supplement: Supplementary file 2 [file appendix-many-register.tex]

\section{Many registers}

% The following lemma shows that flattening termsand unfolding the matrix power commute. 
% \begin{lemma}
%     The following diagram commutes
% \begin{align*}
%     \ranked{
%         \xymatrix{
%             \tmonad \tmonad (\rSigma^{[k]}) \ar[d]_{\flatt_{\rSigma^{[k]}}} \ar[r]^{\tmonad \unfold_{\rSigma}}&
%             \tmonad ( (\tmonad \rSigma)^{[k]}) \ar[d]^{\unfold_{\tmonad \rSigma}} \\
%             \tmonad ( (\tmonad \rSigma)^{[k]}) \ar[r]^{\unfold_{\tmonad \rSigma}} &
%             (\tmonad \rSigma)^{[k]}
%         }
%     }
% \end{align*}
% \end{lemma} 

\begin{lemma}\label{lem:homo-unfold}
    Let $h : \branches \ranked{\Sigma^{[k]}} \to M$ be the function .
    There is a derivable function 
\begin{align*}
    \ranked{
        \xymatrix{
              \tmonad (\rSigma^{[k]})  \ar[r]^{g} & \rSigma^{[k]} 
        }
    }
\end{align*}
which agrees with unfolding over inputs that are $h$-homogeneous.
\end{lemma}
\begin{proof} Consider an input $t \in \ranked{\tmonad (\Sigma^{[k]})}$ that is $h$-homogeneous. By definition, either $t$ has depth at most two, or there is some 
    \begin{align*}
        m : \set{1,\ldots,k} \to \set{1,\ldots,k}
    \end{align*}
    such that all internal subbranches of $t$ have value $m$ under $h$. In the second case, the function $m$ might be surjective or not. We treat these three cases separately, i.e.~depth two, depth at least three  and $m$ surjective, and depth at most three and $m$ non-surjective.
    \begin{center}
        (todo fill in)
    \end{center}
    % \begin{enumerate}
    %     \item The input has depth at most two. To the input 
    %     \begin{align*}
    %         t \in \ranked{\tmonad (\Sigma^{[k]})}
    %     \end{align*}
    %     apply the function 
    %     \begin{align*}
    %         \tmonad (x \mapsto (x,\ldots,x))
    %     \end{align*}
    %     yielding 
    %     \begin{align*}
    %         t_1 \in \ranked{\tmonad (\Sigma^{[k]})}
    %     \end{align*}
    % \end{enumerate}
\end{proof}

\begin{lemma}
    For every $m \in \set{1,2,\ldots}$ there  is a derivable function $\ranked {g^m}$ such that the  diagram  
\begin{align*}
    \ranked{
        \xymatrix{
            \tmonadn m  (\rSigma^{[k]}) \ar[d]_{\flatn m} \ar[dr]^{g^m}\\
            \tmonad (\rSigma^{[k]})  \ar[r]_{\unfold_\rSigma} &  \rSigma^{[k]}
        }
    }
\end{align*}
commutes for inputs  which are hereditarily $h$-homogeneous.
\end{lemma}
\begin{proof}
Induction on $m$. For $m=1$ we use the function from Lemma~\ref{lem:homo-unfold}. For $m >2$, we define  $\ranked{g^m}$ to be the composition
\begin{align*}
    \ranked{
        \xymatrix{
            \tmonad^m (\rSigma^{[k]}) \ar[r]^{\tmonad g^{m-1}} & 
            \tmonad (\rSigma^{[k]}) \ar[r]^g & 
            \rSigma^{[k]}
            } 
    }
\end{align*}
apply first  $\tmonad \ranked{g^{m-1}}$, yielding  to every label 
\end{proof}

\begin{align*}
    \ranked{
        \xymatrix{ \tmonad (\rSigma^{[k]}) \ar[r]^f \ar[rd]_{id}&
            \tmonadn m  (\rSigma^{[k]}) \ar[d]_{\flatn m} \ar[dr]^{g^m}\\ & 
            \tmonad (\rSigma^{[k]})  \ar[r]_{\unfold_\rSigma} & (\tmonad \rSigma)^{[k]}
        }
    }
\end{align*}
